# Supplementary material for: Automatically finding atomic regions for fixing bugs in Concurrent programs
Source: arXiv:1403.1749 source file (2014-03-07)
Supplement: Supplementary file 1 [file appendix.tex]

\appendix
\section{Appendix}
\label{Se:app}
\begin{theorem}
Given a program $P$ with no sequential bugs, \algref{conflictwa} computes a minimal set
$W$ of program points that fixes $P$ when all points $p \in W$ are protected using a weak
atomic section or a global lock. 
\end{theorem}
\IT{proof}. Let us assume that the set $W$ computed by \algref{conflictwa} is not minimal.
Thus, there must exist a point $p$ such that $W \setminus \{p\}$ is a valid solution.
There are two possibilities here.

\IT{Case 1:} $p$ was part of the strong atomicity fix $S$ suggested by \algref{optmhs} and was
fed to \algref{conflictwa} as input.

Since $p$ was part of the strong atomicity fix $S$, \algref{mhs} must have witnessed a set of
buggy traces $t$  which took context switch $p$ and visited a conflicting program point
$p'$. Moreover, it must be the case that $CS(t) \cap S = \{p\}$. In another words, there
must exist a trace $t$ such that of all the context switches $CS(t)$ it took, only $p$ was
part of the strong atomicity fix. If no such trace had been witnessed, it would mean that
for every trace that took a context switch at $p$, there was another context switch  $p''$
which was part of $S$. In this case, $p$ could have been removed from $S$ resulting in a
smaller solution for atomicity fix, a contradiction. This trace $t$ can not be avoided if
$p$ is removed from $W$, since $t$ can still context switch at $p$ and reach the
conflicting program point $p'$ to cause a bug.

\IT{Case 2:} $p$ was not part of $S$, and was added to $W$ by \algref{conflictwa}.

Using the same argument as above, a trace $t$ must exist such that $WCS(t) \cap (W \setminus
S) = \{p\}$. If $p$ is removed from $W$ then $t$ can not be avoided.
